# Supplementary material for: Graph Neural Networks: Architectures, Stability and Transferability
Source: arXiv:2008.01767 source file (2021-01-29)
Supplement: Supplementary file 1 [file ch8_appendix_01_stability_proofs.tex]

% !TEX root = ../compile_all_book/gsp.tex

%%%%%%%%%%%%%%%%%%%%%%%%%%%%%%%%%%%%%%%%%%%%%%%%%%%%%%%
%%%   A   P   P   E   N   D   I   X   %%%%%%%%%%%%%%%%%
%%%%%%%%%%%%%%%%%%%%%%%%%%%%%%%%%%%%%%%%%%%%%%%%%%%%%%%

\section{Stability under Absolute Perturbations}\label{sec_apx_B}

\begin{proof}[Proof of Theorem~\ref{thm:filterStabilityAbsolute}]
Without loss of generality, fix some $\bbP_{0} \in \ccalP_{0}$ and write $\bbP_{0}^{\Tr} \hbS \bbP_{0} = \bbS + \bbE$ for $\bbE \in \ccalE_{A}(\bbS,\hbS)$. Let us start by computing the first order expansion of $(\bbS + \bbE)^{k}$
% eqn
\begin{equation}
    (\bbS + \bbE)^{k} 
        = \bbS^{k} 
            + \sum_{r=0}^{k-1} \bbS^{r} \bbE \bbS^{k-r-1} 
            + \bbC
\end{equation}
with $\bbC$ such that $\|\bbC\|_{2} \leq \sum_{r=2}^{k} \binom{k}{r} \|\bbE\|_{2}^{r} \|\bbS\|_{2}^{k-r}$. Using this first-order approximation in \eqref{eqn:graphFilter}, we get
% eqn
\begin{equation}
    \bbH(\bbP_{0}^{\Tr}\hbS \bbP_{0}) - \bbH(\bbS) = 
        \sum_{k=0}^{\infty} h_{k} 
            \sum_{r=0}^{k-1} 
                \bbS^{r} \bbE \bbS^{k-r-1} 
        + \bbD
\end{equation}
with $\bbD$ such that $\|\bbD\|_{2} = \ccalO(\|\bbE\|^{2})$ since the coefficients $\{h_{k}\}_{k=0}^{\infty}$ of the filter $\bbH(\bbS)$ are defined in terms of the power series expansion of the analytic function $h$ which has bounded derivatives.

Next, consider an arbitrary graph signal $\bbx$ with finite energy $\|\bbx\|_{2}<\infty$ that has a GFT given by $\tbx = [\tdx_{1},\ldots,\tdx_{N}]^{\Tr}$ so that
% eqn
\begin{equation}
    \bbx = \sum_{i=1}^{N} \tdx_{i} \bbv_{i}
\end{equation}
for $\{\bbv_{i}\}_{i=1}^{N}$ the eigenvector basis of the GSO $\bbS$. Then, we can compute
% eqn:filterDifferenceWithXAbsolute
\begin{align} \label{eqn:filterDifferenceWithXAbsolute}
    & \left[ \bbH(\bbP_{0}^{\Tr}\hbS \bbP_{0}) - \bbH(\bbS) \right] \bbx 
          \\
    & \qquad 
        = \sum_{i=1}^{N} \tdx_{i} 
            \sum_{k=0}^{\infty} h_{k} 
                \sum_{r=0}^{k-1} \bbS^{r} \bbE \bbS^{k-r-1} \bbv_{i} + \sum_{i=1}^{N} \tdx_{i} \bbD \bbv_{i}.
      \nonumber
\end{align}
Let us focus on the second term of the sum above. It is immediate that $\bbS^{k-r-1}\bbv_{i} = \lambda_{i}^{k-r-1}\bbv_{i}$, so that
% eqn:allSumEvi
\begin{equation} \label{eqn:allSumEvi}
% aligned
\begin{aligned}
    & \sum_{i=1}^{N} \tdx_{i} 
        \sum_{k=0}^{\infty} h_{k} 
            \sum_{r=0}^{k-1} \bbS^{r} \bbE \bbS^{k-r-1} \bbv_{i} \\
    & \qquad 
        = \sum_{i=1}^{N} \tdx_{i} 
        \sum_{k=0}^{\infty} h_{k} 
            \sum_{r=0}^{k-1} \lambda_{i}^{k-r-1} \bbS^{r} \bbE  \bbv_{i}
\end{aligned}
\end{equation}
Now, using the eigendecomposition of the error $\bbE = \bbU \bbM \bbU^{\Hr}$, we write it as
% algn
\begin{align}
    \bbE & = \bbE_{V} + \bbE _{U} \\
    \bbE_{V} & = \bbV \bbM \bbV^{\Hr} \\
    \bbE_{U} 
        & = \left( \bbU - \bbV \right) \bbM \left( \bbU - \bbV \right)^{\Hr} \\
            & \qquad 
            + \bbV \bbM \left( \bbU - \bbV \right)^{\Hr}
            + \left( \bbU - \bbV \right) \bbM \bbV^{\Hr} \nonumber
\end{align}
so that
% eqn:EviEu
\begin{equation} \label{eqn:EviEu}
    \bbE \bbv_{i} = m_{i} \bbv_{i}+ \bbE_{U} \bbv_{i}.
\end{equation}
Using \eqref{eqn:EviEu} in \eqref{eqn:allSumEvi} yields two terms
% algn
\begin{align}
    & \sum_{i=1}^{N} \tdx_{i} 
        \sum_{k=0}^{\infty} h_{k} 
            \sum_{r=0}^{k-1} \lambda_{i}^{k-r-1} \bbS^{r} \bbE  \bbv_{i} \\
    & = \sum_{i=1}^{N} \tdx_{i} 
        \sum_{k=0}^{\infty} h_{k}
            \sum_{r=0}^{k-1} \lambda_{i}^{k-r-1} \bbS^{r} m_{i}  \bbv_{i} 
                \label{eqn:allSumEviFirstTerm} \\
    & \quad + \sum_{i=1}^{N} \tdx_{i} 
            \sum_{k=0}^{\infty} h_{k}
                \sum_{r=0}^{k-1} \lambda_{i}^{k-r-1} \bbV \bbLam^{r} \bbV^{\Hr} \bbE_{U}  \bbv_{i}.
                \label{eqn:allSumEviSecondTerm}
\end{align}
For \eqref{eqn:allSumEviFirstTerm} we note that $\bbS^{r} \bbv_{i} = \lambda_{i}^{r} \bbv_{i}$, leading to the product $\lambda_{i}^{k-r-1} \lambda_{i}^{r} = \lambda_{i}^{k-1}$ being independent of $r$, so that
% eqn:firstTermSumAbsolute
\begin{equation} \label{eqn:firstTermSumAbsolute}
    \sum_{i=1}^{N} \tdx_{i} m_{i}
        \sum_{k=1}^{\infty} k h_{k} \lambda_{i}^{k-1}  \bbv_{i}
    = \sum_{i=1}^{N} \tdx_{i} m_{i} h'(\lambda_{i}) \bbv_{i}
\end{equation}
where $h'(\lambda_{i}) = \sum_{k=1}^{\infty} k h_{k} \lambda_{i}^{k-1}$ is the derivative $h'(\lambda)$ of $h(\lambda)$ evaluated at $\lambda = \lambda_{i}$. In the case of \eqref{eqn:allSumEviSecondTerm} we note that
% eqn:secondTermSumAbsolute
\begin{equation}\label{eqn:secondTermSumAbsolute}
\begin{aligned} 
    & \sum_{i=1}^{N} \tdx_{i} \bbV
        \sum_{k=0}^{\infty} h_{k} 
            \sum_{r=0}^{k-1} 
                \lambda_{i}^{k-r-1} \bbLambda^{r} \bbV^{\Hr} \bbE_{U} \bbv_{i}  \\
    & \qquad = \sum_{i=1}^{N} \tdx_{i} \bbV
        \diag(\bbg_{i}) \bbV^{\Hr} \bbE_{U} \bbv_{i}
\end{aligned}
\end{equation}
where $\bbg_{i} \in \reals^{N}$ is such that
% eqn
\begin{equation}
    [\bbg_{i}]_{j} 
        = \sum_{k=0}^{\infty} h_{k} 
            \sum_{r=0}^{k-1} \lambda_{i}^{k-r-1} \lambda_{j}^{r}.
\end{equation}
For $j=i$ we have $[\bbg_{i}]_{i} = h'(\lambda_{i})$ while, for $j \neq i$, recall that $\sum_{r=0}^{k-1} \lambda_{i}^{k-r-1}\lambda_{j}^{r} = (\lambda_{i}^{k} - \lambda_{j}^{k})/(\lambda_{i} - \lambda_{j})$ so that
% eqn:giAbsolute
\begin{equation} \label{eqn:giAbsolute}
    [\bbg_{i}]_{j} = 
        \begin{cases}
            h'(\lambda_{i}) 
                & \text{ if} j=i \\
            \frac{h(\lambda_{i})-h(\lambda_{j})}{\lambda_{i}-\lambda_{j}} 
                & \text{ if} j \neq i
        \end{cases}.
\end{equation}
Note $\max_{j} |[\bbg_{i}]_{j}| \leq C_{L}$ due to hypothesis \eqref{eqn:lipschitzFilters}, for all $i=1,\ldots,N$.

Using \eqref{eqn:firstTermSumAbsolute} and \eqref{eqn:secondTermSumAbsolute} back in \eqref{eqn:filterDifferenceWithXAbsolute}, and computing the norm, we get
% eqn
\begin{align}
    & \left\| \left[ \bbH(\bbP_{0}^{\Tr}\hbS \bbP_{0}) - \bbH(\bbS) \right] \bbx \right\|_{2}  \nonumber \\
    & \leq \left\|
        \sum_{i=1}^{N} \tdx_{i} m_{i} h'(\lambda_{i}) \bbv_{i}
           \right\|_{2}
        \label{eqn:firstOrderTermAbsoluteFirstTerm} \\
    & \quad + \left\|   
        \sum_{i=1}^{N} 
            \tdx_{i} \bbV \diag(\bbg_{i}) \bbV^{\Hr} \bbE_{U} \bbv_{i}
           \right\| _{2}
        \label{eqn:firstOrderTermAbsoluteSecondTerm} \\
    & \quad + \left\| \bbD \tbx \right\| _{2}
        \label{eqn:secondOrderTermAbsolute}.
\end{align}
For the first part of the first order term \eqref{eqn:firstOrderTermAbsoluteFirstTerm} we have
% eqn
\begin{equation}
    \left\| \sum_{i=1}^{N} \tdx_{i} m_{i} h'(\lambda_{i}) \bbv_{i} \right\|_{2}^{2}
        = \sum_{i=1}^{N} |\tdx_{i}|^{2} |m_{i}|^{2} |h'(\lambda_{i})|^{2} \| \bbv_{i} \|_{2}^{2}
\end{equation}
since $\{\bbv_{i}\}$ conform an orthonormal basis. Then, we recall that $\|\bbv_{i}\|^{2} = 1$ and, from hypothesis \eqref{eqn:hypothesisEabsolute} we have $|m_{i}| \leq \varepsilon$ and from hypothesis \eqref{eqn:lipschitzFilters}, $|h'(\lambda_{i})| \leq C_{L}$, so that
% eqn
\begin{equation}
    \left\| \sum_{i=1}^{N} \tdx_{i} m_{i} h'(\lambda_{i}) \bbv_{i} \right\|_{2}^{2}
        \leq \varepsilon^{2} C_{L}^{2} \sum_{i=1}^{N} |\tdx_{i}|^{2}.
\end{equation}
Recalling that $\sum_{i=1}^{N} |\tdx_{i}|^{2} = \| \tbx\|_{2}^{2} = \|\bbx\|_{2}^{2}$ and applying square root, we finally bound \eqref{eqn:firstOrderTermAbsoluteFirstTerm} by
% eqn:firstOrderTermAbsoluteFirstTermBound
\begin{equation} \label{eqn:firstOrderTermAbsoluteFirstTermBound}
    \left\| \sum_{i=1}^{N} \tdx_{i} m_{i} h'(\lambda_{i}) \bbv_{i} \right\|_{2}
        \leq \varepsilon C_{L} \| \bbx\|_{2}.
\end{equation}
Now, moving on to \eqref{eqn:firstOrderTermAbsoluteSecondTerm} and using triangle inequality together with submultiplicativity of the operator norm, we have
% eqn:firstOrderTermAbsoluteSecondTermFirstInequality
\begin{equation} \label{eqn:firstOrderTermAbsoluteSecondTermFirstInequality}
% aligned
\begin{aligned}
    & \left\|   
        \sum_{i=1}^{N} \tdx_{i} \bbV \diag(\bbg_{i}) \bbV^{\Hr} \bbE_{U}\bbv_{i} 
    \right\|_{2} \\
        & \qquad \leq 
        \sum_{i=1}^{N}
            |\tdx_{i} |
            \| \bbV \diag(\bbg_{i}) \bbV^{\Hr}\|_{2}
            \|\bbE_{U}\|_{2}
            \|\bbv_{i}\|_{2}. 
        \\
\end{aligned}
\end{equation}
We have $\| \bbV \diag(\bbg_{i}) \bbV^{\Hr}\|_{2} \leq C_{L}$ for all $i=1,\ldots,N$ from \eqref{eqn:giAbsolute} in combination with hypothesis \eqref{eqn:lipschitzFilters}, and also $\|\bbv_{i}\|_{2} = 1$. As for $\|\bbE_{U}\|_{2}$, we note that
% eqn:boundEu
\begin{equation} \label{eqn:boundEu}
% aligned
\begin{aligned}
    \|\bbE_{U}\|_{2} & \leq
        \left\| (\bbU - \bbV) \bbM (\bbU - \bbV)^{\Hr} \right\|_{2} \\
        & \quad 
          + \left\| \bbV \bbM (\bbU - \bbV)^{\Hr} \right\|_{2} 
          + \left\| (\bbU - \bbV) \bbM \bbV^{\Hr} \right\|_{2} \\
        & \leq 
            \| \bbU - \bbV \|_{2}^{2} \| \bbM \|_{2} 
            + 2 \| \bbU - \bbV \|_{2} \| \bbV \|_{2} \| \bbM \|_{2} \\
        & \leq 
            \varepsilon \| \bbU - \bbV \|_{2}^{2} 
            + 2 \varepsilon \| \bbU - \bbV \|_{2}
\end{aligned}
\end{equation}
since $\|\bbE \|_{2} \leq \varepsilon$ by hypothesis \eqref{eqn:hypothesisEabsolute} and $\| \bbV \|_{2} = 1$ for $\bbV$ is an orthonormal matrix. Defining $\varepsilon_{UV} = \| \bbU - \bbV \|_{2}^{2} + 2 \| \bbU - \bbV\|_{2} = (\|\bbU - \bbV\|_{2} + 1)^{2} - 1$ and using \eqref{eqn:boundEu} back in \eqref{eqn:firstOrderTermAbsoluteSecondTermFirstInequality}, we finally get
% eqn:firstOrderTermAbsoluteSecondTermBound
\begin{equation} \label{eqn:firstOrderTermAbsoluteSecondTermBound}
    \left\|   
        \sum_{i=1}^{N} \bbV \diag(\bbg_{i}) \bbV^{\Hr} (\tdx_{i} \bbw_{i}) 
    \right\|_{2}
    \leq
       C_{L} \varepsilon \varepsilon_{UV} \sqrt{N} \| \bbx \|_{2}
\end{equation}
where we used the fact that $\sum_{i=1}^{N} |\tdx_{i} | = \| \tbx_{i} \| _{1} \leq \sqrt{N} \| \tbx \|_{2} = \sqrt{N} \| \bbx\|_{2}$.

Finally, for the second order term \eqref{eqn:secondOrderTermAbsolute} stemming from the expansion of $\bbP_{0}^{\Tr}\hbS^{k} \bbP_{0}$, we obtain 
% eqn:secondOrderTermAbsoluteBound
\begin{equation} \label{eqn:secondOrderTermAbsoluteBound}
    \| \bbD \tbx \|_{2} 
        \leq \ccalO(\| \bbE \|_{2}^{2}) \| \bbx \|_{2} 
        \leq \ccalO(\varepsilon^{2}) \| \bbx \|_{2}.
\end{equation}
Using bound \eqref{eqn:firstOrderTermAbsoluteFirstTermBound} in \eqref{eqn:firstOrderTermAbsoluteFirstTerm} and bound \eqref{eqn:firstOrderTermAbsoluteSecondTermBound} in \eqref{eqn:firstOrderTermAbsoluteSecondTerm}, together with the bound \eqref{eqn:secondOrderTermAbsoluteBound} we just obtained for \eqref{eqn:secondOrderTermAbsolute}, we complete the proof.
\end{proof}

%%%%%%%%%%%%%%%%%%%%%%%%%%%%%%%%%%%%%%%%%%%%%%%%%%%%%%%%%
%%% SECTION : Stability under Relative Perturbations  %%%
%%%%%%%%%%%%%%%%%%%%%%%%%%%%%%%%%%%%%%%%%%%%%%%%%%%%%%%%%

\section{Stability under Relative Perturbations}\label{sec_apx_C}

\begin{proof}[Proof of Theorem~\ref{thm:filterStabilityRelative}]
Without loss of generality, fix some $\bbP_{0} \in \ccalP_{0}$ and write $\bbP_{0}^{\Tr} \hbS \bbP_{0} = \bbS + \bbE^{\Hr} \bbS + \bbS \bbE$. Consider first the computation of the first order expansion of $(\bbA + \bbB)^{k}$ for two square matrices $\bbA$ and $\bbB$
% eqn
\begin{equation}
    (\bbA + \bbB)^{k} 
        = \bbA^{k} 
            + \sum_{r=0}^{k-1} \bbA^{r} \bbB \bbA^{k-r-1} 
            + \bbC
\end{equation}
with $\bbC$ such that $\|\bbC\|_{2} \leq \sum_{r=2}^{k} \binom{k}{r} \|\bbB\|_{2}^{r} \|\bbA\|_{2}^{k-r}$. Using this first-order approximation in \eqref{eqn:graphFilter} with $\bbA = \bbS$ and $\bbB = \bbE^{\Hr} \bbS+ \bbS \bbE$, we get
% eqn
\begin{equation}
% aligned
\begin{aligned}
    & \bbH(\bbP_{0}^{\Tr}\hbS \bbP_{0}) - \bbH(\bbS) \\
    & \quad = 
        \sum_{k=0}^{\infty} h_{k} 
            \sum_{r=0}^{k-1} \left( 
                \bbS^{r} \bbE^{\Hr} \bbS^{k-r} 
                \!\! + \! \bbS^{r+1} \bbE \bbS^{k-r-1} 
            \right)
        + \bbD
\end{aligned}
\end{equation}
with $\bbD$ such that $\|\bbD\|_{2} = \ccalO(\|\bbE\|_{2}^{2})$ since the coefficients $\{h_{k}\}_{k=0}^{\infty}$ of the filter $\bbH(\bbS)$ are defined in terms of the power series expansion of the analytic function $h$ which has bounded derivatives.

Next, consider an arbitrary graph signal $\bbx$ with finite energy $\|\bbx\|_{2}<\infty$ that has a GFT given by $\tbx = [\tdx_{1},\ldots,\tdx_{N}]^{\Tr}$ so that
% eqn
\begin{equation}
    \bbx = \sum_{i=1}^{N} \tdx_{i} \bbv_{i}
\end{equation}
for $\{\bbv_{i}\}_{i=1}^{N}$ the eigenvector basis of the GSO $\bbS$. Then, we can compute
% eqn:filterDifferenceWithX
\begin{align} \label{eqn:filterDifferenceWithX}
    & \left[ \bbH(\bbP_{0}^{\Tr}\hbS \bbP_{0}) - \bbH(\bbS) \right] \bbx 
        = \sum_{i=1}^{N} \tdx_{i} \bbD \bbv_{i} 
    \\
    & \quad + \sum_{i=1}^{N} \tdx_{i} 
        \sum_{k=0}^{\infty} h_{k} 
            \sum_{r=0}^{k-1} \left( 
                \bbS^{r} \bbE^{\Hr} \bbS^{k-r} + \bbS^{r+1} \bbE \bbS^{k-r-1} 
            \right) \bbv_{i}. 
    \nonumber
\end{align}
Let us consider first the product $\bbS^{r+1} \bbE \bbS^{k-r-1} \bbv_{i}$. It is immediate that $\bbS^{k-r-1}\bbv_{i} = \lambda_{i}^{k-r-1}\bbv_{i}$, so we focus on the product
% eqn
\begin{equation}
    \bbE \bbv_{i} 
        = \sum_{n=1}^{N} m_{n} \bbu_{n} \bbu_{n}^{\Hr} \bbv_{i} 
        = m_{N} \sum_{n=1}^{N} 
            \frac{m_{n}}{m_{N}} \bbu_{n} \bbu_{n}^{\Hr} \bbv_{i}.
\end{equation}
The hypothesis \eqref{eqn:hypothesisErelative} that $\| \bbE/m_{N} - \bbI \|_{2} \leq \varepsilon$ is equivalent to $1 - \varepsilon \leq m_{n}/m_{N} \leq 1+\varepsilon$ for all $n = 1,\ldots,N$. Then, we can write $m_{n}/m_{N} = 1+ \delta_{n}$ with $|\delta_{n}| \leq \varepsilon$, which yields
% eqn:Evi
\begin{equation} \label{eqn:Evi}
    \bbE \bbv_{i} 
        = m_{N} \bbv_{i} + m_{N} \bbw_{i} 
    \quad , \quad 
    \bbw_{i} 
        = \sum_{n=1}^{N} \delta_{n} \bbu_{n} \bbu_{n}^{\Hr} \bbv_{i}.
\end{equation}
Note that
% eqn:wiBound
\begin{equation} \label{eqn:wiBound}
    \| \bbw_{i} \|_{2} 
        \leq \left\| \sum_{n=1}^{N} \delta_{n} \bbu_{n} \bbu_{n}^{\Hr} \right\|_{2} 
                  \| \bbv_{i} \|_{2} 
    = \max_{n=1,\ldots,N} |\delta_{n}| 
        \leq \varepsilon.
\end{equation}

Using \eqref{eqn:Evi} we get that
% eqn
\begin{equation}
    \bbS^{r+1} \bbE \bbS^{k-r-1} \bbv_{i} 
        = m_{N} \lambda_{i}^{k} \bbv_{i} 
            + m_{N} 
                \bbV \lambda_{i}^{k-r-1} \bbLambda^{r+1} \bbV^{\Hr} 
                \bbw_{i}.
\end{equation}
And this can be used to compute
% eqn:termE
\begin{equation} \label{eqn:termE}
% aligned
\begin{aligned}
    & \sum_{k=0}^{\infty} h_{k} 
        \sum_{r=0}^{k-1} \bbS^{r+1} \bbE \bbS^{k-r-1} \bbv_{i} 
    = m_{N} \sum_{k=0}^{\infty} h_{k} (k \lambda_{i}^{k} \bbv_{i})
    \\
    & \quad + m_{N} \bbV 
        \left( \sum_{k=0}^{\infty} h_{k} 
            \sum_{r=0}^{k-1} \lambda_{i}^{k-r-1} \bbLambda^{r+1} 
        \right) 
            \bbV^{\Hr} \bbw_{i} 
    \\
    & = m_{N} \lambda_{i} h'(\lambda_{i}) \bbv_{i} 
        + m_{N} \bbV \diag(\hbg_{i}) \bbV^{\Hr} \bbw_{i}
\end{aligned}
\end{equation}
where vector $\hbg_{i} \in \reals^{N}$ is such that
% eqn
\begin{equation}
    [\hbg_{i}]_{j} = 
        \sum_{k=0}^{\infty} h_{k} 
            \sum_{r=0}^{k-1} \lambda_{i}^{k-r-1} \lambda_{j}^{r+1}.
\end{equation}
We note that if $j=i$ then $\lambda_{i}^{k-r-1} \lambda_{j}^{r+1} = \lambda_{i}^{k}$ and thus $[\hbg_{i}]_{i} = \lambda_{i} h'(\lambda_{i})$. For $j \neq i$, on the other hand, noting that $\sum_{r=0}^{k-1} \lambda_{i}^{k-r-1} \lambda_{j}^{r+1} = \lambda_{j} (\lambda_{i}^{k} - \lambda_{j}^{k})/(\lambda_{i}-\lambda_{j})$ we have
% eqn
\begin{equation}
    [\hbg_{i}]_{j} 
        = \sum_{k=0}^{\infty} h_{k} 
            \lambda_{j} 
            \frac{\lambda_{i}^{k} - \lambda_{j}^{k}}{\lambda_{i} - \lambda_{j}}
        = \frac{\lambda_{j}}{\lambda_{i}-\lambda_{j}} 
            \sum_{k=0}^{\infty} h_{k} 
                \left(\lambda_{i}^{k} - \lambda_{j}^{k} \right).
\end{equation}
Therefore,
% eqn:hatg
\begin{equation} \label{eqn:hatg}
    [\hbg_{i}]_{j} = 
        \begin{cases}
            \lambda_{i} h'(\lambda_{i}) 
                & \text{if } j=i \\
            \lambda_{j} 
            \frac{h(\lambda_{i}) - h(\lambda_{j})}{\lambda_{i}-\lambda_{j}}
                & \text{if } j \neq i
        \end{cases}
\end{equation}
We also observe that $|[\hbg_{i}]_{j}| \leq G \lesssim \max\{C, 2B\}$ for all $j=1,\ldots,N$ due to the fact that $|h(\lambda)| \leq B$ and $|\lambda h'(\lambda)| \leq C$ as per hypothesis \eqref{eqn:integralLipschitzFilters}.

We can get an expression analogous to \eqref{eqn:termE} for the term
% eqn:termEH
\begin{equation} \label{eqn:termEH}
% aligned
\begin{aligned}
\sum_{k=0}^{\infty} h_{k} & \sum_{r=0}^{k-1} \bbS^{r} \bbE^{\Hr} \bbS^{k-r} \bbv_{i} \\
& = m_{N} \lambda_{i} h'(\lambda_{i})\bbv_{i} + m_{N} \bbV \diag(\check{\bbg}_{i}) \bbV^{\Hr} \bbw_{i}
\end{aligned}
\end{equation}
where now
% eqn:checkg
\begin{equation} \label{eqn:checkg}
    [\check{\bbg}_{i}]_{j} = 
        \begin{cases}
            \lambda_{i} h'(\lambda_{i}) 
                & \text{if } j=i \\
            \lambda_{i} 
            \frac{h(\lambda_{i}) - h(\lambda_{j})}{\lambda_{i}-\lambda_{j}}
                & \text{if } j \neq i
        \end{cases}
\end{equation}
where it also holds that $|[\check{\bbg}_{i}]_{j}| \leq G$.

Finally, using \eqref{eqn:termE} and \eqref{eqn:termEH} back in \eqref{eqn:filterDifferenceWithX}, and applying the norm, we get
% eqn
\begin{align}
    & \left\| \left[ \bbH(\bbP_{0}^{\Tr}\hbS \bbP_{0}) - \bbH(\bbS) \right] \bbx \right\|_{2}  
        \nonumber \\
    & \leq \left\| 2 m_{N} 
        \sum_{i=1}^{N} \lambda_{i}h'(\lambda_{i}) \tdx_{i} \bbv_{i}  
        \right\|_{2}
        \label{eqn:firstOrderTerm} \\
    & \quad + \left\| m_{N}  
        \sum_{i=1}^{N} 
            \bbV \diag(\hbg_{i}+ \check{\bbg}_{i}) \bbV^{\Hr} 
            (\tdx_{i} \bbw_{i}) 
        \right\|_{2} 
        \label{eqn:secondOrderTermEvi} \\
    & \quad + \left\| \bbD \tbx \right\|_{2} 
        \label{eqn:secondOrderTermTaylor}.
\end{align}
For the first order term \eqref{eqn:firstOrderTerm} we have
% eqn
\begin{equation}
    \left\| 2 m_{N} 
        \sum_{i=1}^{N} 
            \lambda_{i}h'(\lambda_{i}) 
            \tdx_{i} \bbv_{i} 
        \right\|_{2}^{2} 
    = 4 |m_{N}|^{2} 
        \sum_{i=1}^{N} 
            |\lambda_{i} h'(\lambda_{i})|^{2}
            |\tdx_{i}|^{2}
\end{equation}
since $\{\bbv_{i}\}_{i=1}^{N}$ form an orthonormal basis. Then, bounding $|m_{N}| \leq \varepsilon/2$ in virtue of \eqref{eqn:hypothesisDistanceRelative} and $|\lambda h'(\lambda)| \leq C$ for all $\lambda$ as per \eqref{eqn:integralLipschitzFilters}, we get
% eqn:boundFirstOrderTerm
\begin{equation} \label{eqn:boundFirstOrderTerm}
    4 |m_{N}|^{2} 
        \sum_{i=1}^{N} |\lambda_{i} h'(\lambda_{i})|^{2} |\tdx_{i}|^{2} 
    \leq \varepsilon^{2} C^{2} 
        \sum_{i=1}^{N} |\tdx_{i}|^{2} 
    = \varepsilon^{2} C^{2} \| \bbx \|_{2}^{2}.
\end{equation}
For the second order term \eqref{eqn:secondOrderTermEvi} coming from $\bbE \bbv_{i}$, we have
% eqn
\begin{equation}
% aligned
\begin{aligned}
    & \left\| m_{N}  
        \sum_{i=1}^{N}
            \bbV \diag(\hbg_{i}+ \check{\bbg}_{i}) \bbV^{\Hr} 
            (\tdx_{i} \bbw_{i}) \right\|_{2} 
    \\
    & \leq |m_{N}|
        \sum_{i=1}^{N} 
            \| \bbV \diag(\hbg_{i}+ \check{\bbg}_{i}) \bbV^{\Hr}\|_{2}
            |\tdx_{i} | \|\bbw_{i}\|_{2}
\end{aligned}
\end{equation}
where, by bounding $|m_{N}| \leq \varepsilon/2$ using \eqref{eqn:hypothesisDistanceRelative}, $\| \bbV \diag(\hbg_{i}+ \check{\bbg}_{i}) \bbV^{\Hr} \|_{2} \leq 2G$ in virtue of \eqref{eqn:hatg} and \eqref{eqn:checkg}, $\sum_{i=1}^{N} |\tdx_{i}| = \| \tbx \|_{1} \leq \sqrt{N} \|\tbx\|_{2} = \sqrt{N} \|\bbx\|_{2}$ and $\|\bbw_{i}\|_{2} \leq \varepsilon$ because of \eqref{eqn:wiBound}, we get
% eqn:boundSecondOrderTermEvi
\begin{equation} \label{eqn:boundSecondOrderTermEvi}
    \left\| m_{N}  
        \sum_{i=1}^{N}
        \bbV \diag(\hbg_{i}+ \check{\bbg}_{i}) \bbV^{\Hr}
        (\tdx_{i} \bbw_{i}) 
    \right\|_{2}
    \leq \ccalO(\varepsilon^{2}) \| \bbx \|_{2}.
\end{equation}
Finally, for the second order term \eqref{eqn:secondOrderTermTaylor} stemming from the expansion of $\bbP_{0}^{\Tr}\hbS^{k} \bbP_{0}$, we obtain 
% eqn:boundSecondOrderTermTaylor
\begin{equation} \label{eqn:boundSecondOrderTermTaylor}
    \| \bbD \tbx \|_{2} \leq \ccalO(\| \bbE \|_{2}^{2}) \| \bbx \|_{2} 
        \leq \ccalO(\varepsilon^{2}) \| \bbx \|_{2}.
\end{equation}
Using bounds \eqref{eqn:boundFirstOrderTerm}, \eqref{eqn:boundSecondOrderTermEvi} and \eqref{eqn:boundSecondOrderTermTaylor} back in \eqref{eqn:firstOrderTerm}, \eqref{eqn:secondOrderTermEvi} and \eqref{eqn:secondOrderTermTaylor}, respectively, we complete the proof.
\end{proof}

%%%%%%%%%%%%%%%%%%%%%%%%%%%%%%%%%%%%%%%%%%%%%%%%%%%
%%% SECTION : Permutation Equivariance of GNNs  %%%
%%%%%%%%%%%%%%%%%%%%%%%%%%%%%%%%%%%%%%%%%%%%%%%%%%%

\section{Permutation Equivariance of GNNs}

\begin{proof}[Proof of Proposition~\ref{prop:GNNPermutationEquivariance}]
Let us first consider layer $1$, evaluating it on $\hbS$
% eqn:layerOneOnHatS
\begin{equation} \label{eqn:layerOneOnHatS}
    \bbx^{f}_{1}(\hbS) = \sigma_{1} 
        \left( 
            \sum_{g=1}^{F_{0}}
                \bbH^{fg}_{1}(\hbS) \bbP^{\Tr} \bbx^{g}
        \right)
        =
        \sigma_{1} \left( \bbP^{\Tr}
            \sum_{g=1}^{F_{0}}
                \bbH^{fg}_{1}(\bbS) \bbx^{g}
        \right)
\end{equation}
where we have used Prop.~\ref{prop:filterPermutationEquivariance} on filter $\bbH^{fg}_{1}$. Now, since $\sigma_{1}$ is pointwise, then it holds that $\sigma_{1}(\bbP^{\Tr} \bbz) = \bbP^{\Tr} \sigma_{1}(\bbz)$ for all $\bbz \in \reals^{N}$, so that
% eqn
\begin{equation}
    \bbx_{1}^{f}(\hbS) = \bbP^{\Tr} \bbx_{1}^{f}(\bbS)
\end{equation}
Next, consider an arbitrary layer of the GNN [cf. \eqref{eqn:GNN}]
% eqn:arbitraryLayer
\begin{equation} \label{eqn:arbitraryLayer}
    \bbx^{f}_{\ell}(\bbS) = \sigma_{\ell} 
        \left( 
            \sum_{g=1}^{F_{\ell-1}}
                \bbH^{fg}_{\ell}(\bbS) \bbx^{g}_{\ell-1}(\bbS)
        \right)
\end{equation}
and assume that $\bbx_{\ell-1}^{g}(\hbS) = \bbP^{\Tr} \bbx_{\ell-1}^{g}(\bbS)$ for all $g=1,\ldots,F_{\ell-1}$. Then, by evaluating layer \eqref{eqn:arbitraryLayer} on $\hbS = \bbP^{\Tr} \bbS \bbP$, together with Prop.~\ref{prop:filterPermutationEquivariance} on filters $\bbH_{\ell}^{fg}$, we get
% eqn:arbitraryLayerOnHatS
\begin{equation} \label{eqn:arbitraryLayerOnHatS}
% aligned
\begin{aligned}
    \bbx^{f}_{\ell}(\hbS)& = \sigma_{\ell} 
        \left( 
            \sum_{g=1}^{F_{\ell-1}}
            \bbH^{fg}_{\ell}(\hbS) \bbx^{g}_{\ell-1}(\hbS)
        \right) \\
     & = \sigma_{\ell} 
        \left( \bbP^{\Tr} 
            \sum_{g=1}^{F_{\ell-1}}
                \bbH^{fg}_{\ell}(\bbS) \bbP \bbP^{\Tr} \bbx^{g}_{\ell-1}(\bbS)
        \right) \\
     & = \sigma_{\ell} 
         \left( \bbP^{\Tr} 
             \sum_{g=1}^{F_{\ell-1}}
                 \bbH^{fg}_{\ell}(\bbS) \bbx^{g}_{\ell-1}(\bbS)
         \right)
\end{aligned}
\end{equation}
Using the equivariance of the pointwise nonlinearity, we prove that
% eqn
\begin{equation}
    \bbx_{\ell}^{f}(\hbS) = \bbP^{\Tr} \bbx_{\ell}^{f}(\bbS)
\end{equation}
holds for $\ell$, whenever it holds for $\ell-1$. Finally, since it holds for $\ell=1$, then it also holds for $\ell=L$ and therefore it holds for $\hby^{f}(\hbS) = \bbx_{L}^{f}(\hbS)$ for all $f=1,\ldots,F_{L}$, completing the proof.
\end{proof}

%%%%%%%%%%%%%%%%%%%%%%%%%%%%%%%%%%%%
%%% SECTION : Stability of GNNs  %%%
%%%%%%%%%%%%%%%%%%%%%%%%%%%%%%%%%%%%

\section{Graph Neural Networks Stability}

\begin{proof}[Proof of Theorem~\ref{thm:GNNStability}]
Without loss of generality, assume $\bbP_{0} \in \ccalP_{0}$ and write $\bbP_{0}^{\Tr} \hbS \bbP_{0} = \bbS + \bbE^{\Hr} \bbS + \bbS \bbE$. Without any further loss of generality, assume $\bbP_{0} = \bbI$\footnote{To see this, just rename $\bbP_{0}^{\Tr} \hbS \bbP_{0}$ as $\hbS$ and follow the rest of the proof.}. By definition of $\|\hby(\bbS)\|_{2}^{2}$, we have
% eqn:ineqyGNN
\begin{equation} \label{eqn:ineqyGNN}
    \| \hby(\bbS) - \hby(\hbS) \|_{2}^{2} 
        = \sum_{f=1}^{F_{L}} \| \hby^{f}(\bbS) - \hby^{f}(\hbS) \|_{2}^{2}.
\end{equation}
Now, focusing on one of the features
% eqn
\begin{equation}
% aligned
\begin{aligned}
    & \| \hby^{f}(\bbS) - \hby^{f}(\hbS) \|_{2} 
        = \| \bbx_{L}^{f}(\bbS) - \bbx_{L}^{f}(\hbS) \|_{2}
    \\
    & \quad = \left\| 
        \sigma \left( 
            \sum_{g=1}^{F_{L-1}} \bbH_{L}^{fg} (\bbS) \bbx_{L-1}^{g}(\bbS) 
         \right) 
         \right.
    \\
    & \qquad \qquad \left.
         - \sigma \left( 
            \sum_{g=1}^{F_{L-1}} \bbH_{L}^{fg} (\hbS) \bbx_{L-1}^{g}(\hbS) 
        \right) 
        \right\|_{2}
\end{aligned}
\end{equation}
and applying Lipschitz continuity of the nonlinearity \eqref{eqn:lipschitzNonlinearityGNN}, followed by the triangular inequality, we get
% eqn:diffLf
\begin{equation} \label{eqn:diffLf}
% aligned
\begin{aligned}
    & \| \bbx_{L}^{f} (\bbS) - \bbx_{L}^{f}(\hbS) \|_{2} 
        \\
    & \leq C_{\sigma} 
        \sum_{g=1}^{F_{L-1}} 
            \left\| \bbH_{L}^{fg}(\bbS) \bbx_{L-1}^{g}(\bbS) 
                - \bbH_{L}^{fg}(\hbS) \bbx_{L-1}^{g}(\hbS) \right\|_{2}.
\end{aligned}
\end{equation}
Adding and subtracting $\bbH_{L}^{fg}(\hbS) \bbx_{L-1}^{fg}(\bbS)$ from the terms in the sum, and using the triangular inequality once more, we get
% align
\begin{align}
    & \left\| \bbH_{L}^{fg}(\bbS) \bbx_{L-1}^{g}(\bbS) 
        - \bbH_{L}^{fg}(\hbS) \bbx_{L-1}^{g}(\hbS) \right\|_{2} \\
    & \qquad \leq \left\| 
        \left(\bbH_{L}^{fg}(\bbS) - \bbH_{L}^{fg}(\hbS) \right) 
            \bbx_{L-1}^{g}(\bbS) 
        \right\|_{2} 
    \\
    & \qquad \qquad 
        + \left\| \bbH_{L}^{fg}(\hbS) 
            \left( \bbx_{L-1}^{g}(\bbS) - \bbx_{L-1}^{g}(\hbS) \right) 
          \right\|_{2}.
\end{align}
The definition of operator norm, implies that
% align
\begin{align}
& \left\| \bbH_{L}^{fg}(\bbS) \bbx_{L-1}^{g}(\bbS) 
- \bbH_{L}^{fg}(\hbS) \bbx_{L-1}^{g}(\hbS) \right\|_{2} \label{eqn:diffLfg}\\
& \qquad \leq \left\| \bbH_{L}^{fg}(\bbS) - \bbH_{L}^{fg}(\hbS) \right\|_{2} 
\left\| \bbx_{L-1}^{g}(\bbS) \right\|_{2} \label{eqn:normL-1} \\
& \qquad \qquad + \left\| \bbH_{L}^{fg}(\hbS) \right\|_{2}
\left\| \bbx_{L-1}^{g}(\bbS) - \bbx_{L-1}^{g}(\hbS) \right\|_{2} \label{eqn:boundL-1}.
\end{align}
We note that the hypothesis of Theorem \ref{thm:filterStabilityRelative} are satisfied for all $f$, $g$ and $\ell$, and as such, $\| \bbH_{L}^{fg}(\bbS) - \bbH_{L}^{fg}(\hbS) \|_{\ccalP} \leq \varepsilon C$. Also, from hypothesis \eqref{eqn:filterFrameGNN}, we have $\|\bbH_{L}^{fg} (\hbS) \|_{2} \leq B$. Using these two facts on \eqref{eqn:normL-1} and \eqref{eqn:boundL-1}, respectively, and substituting \eqref{eqn:diffLfg} back in \eqref{eqn:diffLf}, we get
% align
\begin{align} \label{eqn:boundL}
    & \| \bbx_{L}^{f}(\bbS) - \bbx_{L}^{f}(\hbS) \|_{2} 
    \\
    & \leq C_{\sigma} 
        \sum_{g=1}^{F_{L-1}} 
            \left( 
                \varepsilon C \| \bbx_{L-1}^{g}(\bbS) \|_{2} 
                + B \| \bbx_{L-1}^{g}(\bbS) - \bbx_{L-1}^{g}(\hbS) \|_{2} 
            \right).
    \nonumber
\end{align}

We observe that \eqref{eqn:boundL} shows a recursion, where the bound at layer $L$ depends on the bound at layer $L-1$ as well as the norm of the features at layer $L-1$, summed over all features. That is, for an arbitrary layer $\ell = 1,\ldots,L$, we have
% align
\begin{align} \label{eqn:boundell}
    & \| \bbx_{\ell}^{f}(\bbS) - \bbx_{\ell}^{f}(\hbS) \|_{2} 
    \\
    & \leq C_{\sigma} 
        \sum_{g=1}^{F_{\ell-1}} 
            \left( 
                \varepsilon C \| \bbx_{\ell-1}^{g}(\bbS) \|_{2} 
                + B \| \bbx_{\ell-1}^{g}(\bbS) - \bbx_{\ell-1}^{g}(\hbS) \|_{2} 
            \right).
        \nonumber
\end{align}
with initial conditions given by the input features $\{\bbx^{g}\}_{g=1}^{F_{0}}$, i.e. $\| \bbx_{0}^{g}(\bbS) \|_{2} = \| \bbx^{g}\|_{2}$ and $\| \bbx_{0}^{g}(\bbS) - \bbx_{0}^{g}(\hbS)\|_{2} = \|\bbx^{g} - \bbx^{g} \|_{2} = 0$. For the first step to solve the recursion \eqref{eqn:boundL}, we compute the norm $\|\bbx_{\ell}^{g}(\bbS)\|_{2}$. We observe that
% eqn:recursionNorm
\begin{equation} \label{eqn:recursionNorm}
    \| \bbx_{\ell}^{f}(\bbS) \|_{2} 
        = \left\| 
            \sum_{g=1}^{F_{\ell-1}} 
                \bbH_{\ell}^{fg}(\bbS) \bbx_{\ell-1}^{g}(\bbS) 
            \right\|_{2} 
       \leq B \sum_{g=1}^{F_{\ell-1}} \| \bbx_{\ell-1}^{g}(\bbS) \|_{2}
\end{equation}
where we used the triangle inequality, followed by hypothesis \ref{eqn:filterFrameGNN} on the filters. Solving recursion \eqref{eqn:recursionNorm} with initial condition $\|\bbx_{0}^{g}\|_{2} = \| \bbx^{g}\|_{2}$ yields
% eqn:solutionNorm
\begin{equation} \label{eqn:solutionNorm}
    \| \bbx_{\ell}^{f} (\bbS) \|_{2} 
        \leq B^{\ell} 
            \prod_{\ell'=1}^{\ell-1} F_{\ell'} 
                \sum_{g=1}^{F_{0}} \| \bbx^{g} \|_{2}.
\end{equation}
Using \eqref{eqn:solutionNorm} back in recursion \eqref{eqn:boundell} and solving it with the corresponding initial conditions, we get
% eqn:solutionBound
\begin{equation} \label{eqn:solutionBound}
    \left\| \bbx_{\ell}^{f} (\bbS) - \bbx_{\ell}^{f}(\hbS) \right\|_{2}
        \leq \varepsilon B^{\ell-1} C 
            \sum_{\ell'=1}^{\ell} 
                C_{\sigma}^{\ell'} 
                \prod_{\ell'=1}^{\ell-1}F_{\ell'} 
                    \sum_{g=1}^{F_{0}} \| \bbx^{g} \|_{2}.
\end{equation}
Evaluating \eqref{eqn:solutionBound} for $\ell=L$ and using it back in \eqref{eqn:boundL}, we get that \eqref{eqn:ineqyGNN} yields
% eqn:finalBoundL
\begin{equation} \label{eqn:finalBoundL}
% aligned
\begin{aligned}
    & \left\| \hby(\bbS) - \hby(\hbS) \right\|_{2}^{2} 
        = \sum_{f=1}^{F_{L}} \left\| 
            \bbx_{L}^{f}(\bbS) - \bbx_{L}^{f}  (\hbS) 
          \right\|_{2}^{2} 
    \\
    & \quad \leq 
        \sum_{f=1}^{F_{L}} \left( 
            \varepsilon B^{L-1} C 
            \sum_{\ell=1}^{L} C_{\sigma}^{\ell} 
                \prod_{\ell=1}^{L-1}F_{\ell} 
            \sum_{g=1}^{F_{0}} \| \bbx^{g} \|_{2}
        \right)^{2}.
\end{aligned}
\end{equation}
Noting that no term in the sum of \eqref{eqn:finalBoundL} depends on $f$, and subsequently applying a square root, we complete the proof.
\end{proof}

\begin{proof}[Proof of corollary \ref{cor:singleLayerStability}]
This follows straight from \eqref{eqn:stabilityBoundGNN} in Theorem~\ref{thm:GNNStability} by setting $F_{0}=1$ and noting that, then, $\sum_{g=1}^{1} \| \bbx^{g} \|_{2} = \|\bbx\|_{2}$.
\end{proof}
